# Supplementary material for: Category-Extensible Out-of-Distribution Detection via Hierarchical Context Descriptions
Source: arXiv:2407.16725 source file (2024-11-14)
Supplement: Supplementary file 1 [file 3_cmp.tex]

\section{Novelty Justification}

Since the CoOp~\cite{zhou2022coop} framework was proposed, vision-language prompt-tuning has been widely studied to leverage the large-scale pre-trained CLIP~\cite{radford2021clip} model. 
The research scope involves few-shot learning~\cite{zhou2022conditional,lu2022prompt}, dense prediction~\cite{rao2022denseclip,du2022learning}, video recognition~\cite{ju2022prompting,gao2023compositional}, \etc~
Among them, DualCoOp~\cite{sun2022dualcoop} shares some similarity with our method.
Specifically, it also learns a ``negative'' context for each category.
However, we have different motivations.
Designed for multi-label recognition, DualCoOp takes the negative contexts to describe the \textit{background} area and focuses on spatial predictions (\ie, object localization), whose idea is similar to YOLO series~\cite{redmon2016you,redmon2018yolov3}.
Instead, our proposed \mmethod~deals with the open-world multi-category classification problem, where the spurious context is developed to describe the latent \textit{spurious category} for a certain ID category, and integrate with the perceptual context to hierarchically describe a precise category boundary.
Besides, if we simply use the maximum binary probability~\cite{hendrycks2019benchmark} (\ie, $\gamma$ in Eq.(5)) as DualCoOp for OOD detection, the performance dramatically decreases, as shown in ~\cref{tab:dualcoop}.
It signifies the necessity to leverage the hierarchical perceptual and spurious contexts to describe category boundaries.

\begin{table}[h]
  \centering
  \small
  \caption{Comparison between DualCoOp and our method.}
  \begin{tabular}{ccc}
    \toprule
    Method & FPR95$\downarrow$ & AUROC$\uparrow$  \\
    \midrule
    DualCoOp~\cite{sun2022dualcoop}       & 28.82 & 95.00 \\
    \textbf{\mmethod}~(Ours)             & \topa{10.31} & \topa{97.82} \\
    \bottomrule
  \end{tabular} 
  \label{tab:dualcoop}
\end{table}

Recently, large language models (LLMs) like GPT-3~\cite{brown2020language} have seen remarkable successes as implicit knowledge bases~\cite{petroni2019language}. Instead of a single category name, one may query LLMs for more visual descriptions with natural language of each ID category, and perform close-set classification~\cite{menon2022visual}. 
When it comes to the open-world setting, how to generate descriptions for unseen categories is still challenging.
Simply generating several candidate OOD descriptions is hard to obtain satisfactory OOD performance~\cite{esmaeilpour2022zero,fort2021exploring,ming2022mcm}, while \cref{tab:perturb_infer} indicates manually perturbing the visual characters for ID descriptions is inefficient in detecting OOD samples as well.
Therefore, we suggest that automatically learning the hierarchical descriptions should be more effective, and we leave the integration with LLMs as future work.
